# Supplementary material for: Experimentally measuring rolling and sliding in three-dimensional dense granular packings
Source: arXiv:2108.11975 source file (2022-08-03)
Supplement: Supplementary file 1 [file supporting_info_final.pdf]

# Supplemental Material for "Experimentally measuring rolling and sliding in three-dimensional dense granular packings"

## I. INFERENCE OF GRAINS' POSITIONS AND ORIENTATIONS

We infer grain positions by convolving the three-dimensional stack of images with a modified three-dimensional Gaussian kernel [1]. Wherever the convolution yields a large value (above a predetermined threshold) in the three-dimensional image lies a candidate grain. Due to the anisotropy introduced into a grain by the two cavities, some candidates are not true grains—are what we call "fake." To distinguish real grains, we use a deep-learning model called a variational autoencoder [2, 3]. A variational autoencoder has a bottleneck structure, consisting of an encoder, a small latent space, and a decoder. The encoder, as well as the decoder, is a dense neural network of two hidden layers. The encoder compresses input data to a low-dimensional latent space in which each coordinate represents a probability distribution's mean. The decoder samples from these distributions in an attempt to reconstruct the original input. By forcing the input through the latent-space bottleneck, the variational autoencoder extracts the input's most meaningful features [4].

Our input is a 25 × 25 × 25 subimage that the Gaussian kernel identified as a candidate bead. We train the variational autoencoder on all the candidate beads in two experimental images—approximately 40,000 fake and real inputs, total. The encoder compresses each candidate bead to a point in a two-dimensional latent space (Fig. 2). The latent space divides clearly into two regions, which represent false (blue) and real (red) beads. The right-hand side of Fig. 2 shows the corresponding candidate beads' outlines in the experimental image. This novel technique, whose training is unsupervised, provides an efficient means of distinguishing correct and incorrect particle identifications.

We infer the grains' orientations after locating the particles' centers. As shown in Fig. 7, we apply a rotating Laplacian-of-a-Gaussian (LoG) filter. The filter is constructed according to the equation

$$f(x, y, z) = (x^2 + y^2 - \sigma^2)e^{-\frac{x^2+y^2}{2\sigma^2}} g(z), \tag{1}$$

wherein

$$g(z) = e^{(z-2\sigma_z)^2/(2\sigma_z^2)} + e^{(z+2\sigma_z)^2/(2\sigma_z^2)}. \tag{2}$$

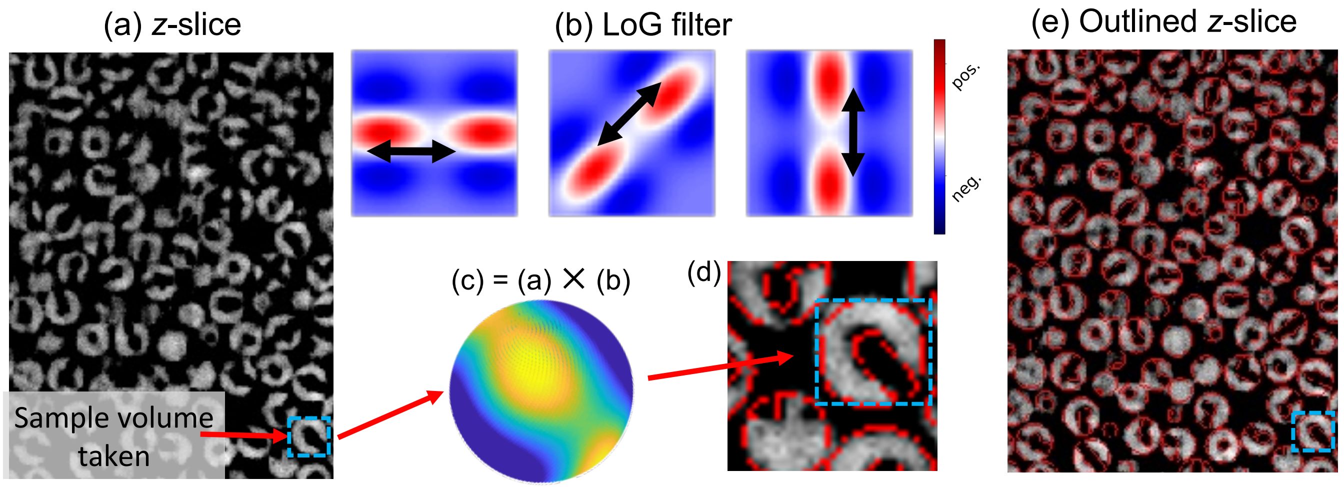


Figure 1. (a) Zoomed-in slice, along the $z$-axis, of grains that contain two holes each. Inset: Sample region used in the rotating convolution. (b) Selected orientations of the modified LoG filter that are used to extract the orientations. (c) Surface map of the convolution, for one grain, with the LoG filter. (d) Zoomed-in $z$-slice, and (e) original $z$-slice, with the grains' extracted positions and orientations shown in red.

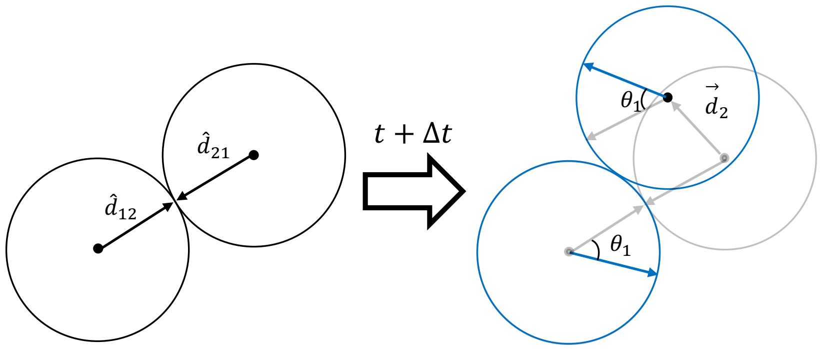


Figure 2. Schematic of the quantities used to calculate the sliding and rolling displacements of two grains in contact. The final-frame displacements (blue circles) show the center-of-mass motion $\vec{d_i}$. The blue arrows show the rotation of each grain's center of mass through an angle $\theta_i$. The initial contact point is denoted by $\hat{d}_{12}$. The rotation axis $\hat{a}_i$ points out of the paper.

The spatial coordinates are denoted by $x$, $y$, and $z$. $\sigma$ denotes the bead's radius in pixels, and $\sigma_z = \frac{1}{2}(\sigma + r_{\text{cyl}})$. $r_{\text{cyl}}$ denotes the cylindrical cavity's radius in pixels.

The $xy$ portion of the equation models cylindrical shapes. Since each bead has two holes, we introduce $f(z)$ to account for the second perpendicular cavity. This function has two peaks away from the bead's center, sharpening the convolution to align exactly with both cavities. To find the bead's orientation, we rotate the $z$-axis uniformly on a unit sphere. The resulting convolution is a map defined on the unit sphere, as shown in Fig. 7. The two axes are clearly visible as maxima for select orientations.

## II. CALCULATING ROTATIONAL AND SLIDING DISPLACEMENTS

The rotational displacements are calculated using the Kabsch algorithm [5]. Let $\hat{p}$ denote the orientation attributed to a grain in one snapshot, and let $\hat{q}$ denote the orientation inferred from the next snapshot. The algorithm features the covariance-like matrix

$$C = \begin{pmatrix}\hat{p}_0 & \hat{q}_0\end{pmatrix} \cdot \begin{pmatrix}\hat{p}_1 \\ \hat{q}_1\end{pmatrix}. \tag{3}$$

The covariance-like matrix has a singular-value decomposition

$$C = U\Sigma V^T. \tag{4}$$

$U$ and $V$ denote the left and right singular vectors. $\Sigma$ denotes a diagonal matrix whose diagonal contains the singular values. The rotation matrix is a product of the singular vectors:

$$R = VU^T. \tag{5}$$

The rotational displacement is $2\cos\theta = \text{Tr}(R) - 1$. The axis of rotation, $a$, is defined by the off-diagonal components of $R + R^{-1}$. The sliding and rolling displacements are computed from [6]:

$$\Delta_{\text{sld}} = |(\vec{d_1} - \vec{d_2}) + (r\theta_1\hat{a}_1 \times \hat{d}_{12} - r\theta_2\hat{a}_2 \times \hat{d}_{21})| \tag{6}$$

and

$$\Delta_{\text{roll}} = \frac{1}{2}r|(\theta_1\hat{a}_1 - \theta_2\hat{a}_2) \times \hat{d}_{12}|. \tag{7}$$

The subscripts 1 and 2 label the two grains that meet at a contact. $\vec{d_i}$ denotes the displacement vector of grain $i$. $\hat{a}_i$, $\theta_i$, and $r$ denote sphere $i$'s rotation axis, angle, and radius. $\hat{d}_{12}$ denotes the unit vector corresponding to the contact normal from grain 1 to 2. Figure 8 shows a schematic of all of these quantities in a two-dimensional projection.

Figure S4 shows the analogue to Fig. 5 calculated with the simulations. We see good agreement for all types of motion observed. Evidently, the only discrepency is the larger amount of translations at the extremes of the Cycle. This could be due to the softness of the spheres used in the simulations compared to the experiments. In the experiments, the grains' have a stiffness many orders of magnitude above what is feasible in MD simulations. However, the softness chosen ($< 1\%$ overlap) is sufficient to model our experimental results and infer energy dissipation from the simulations.

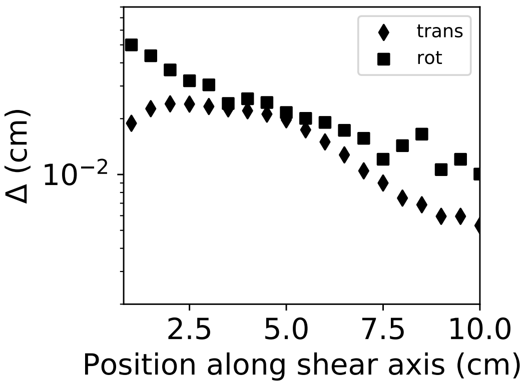


Figure 3. Translations corrected for a linear strain plotted along with the rotations as a function of position along the shear axis.

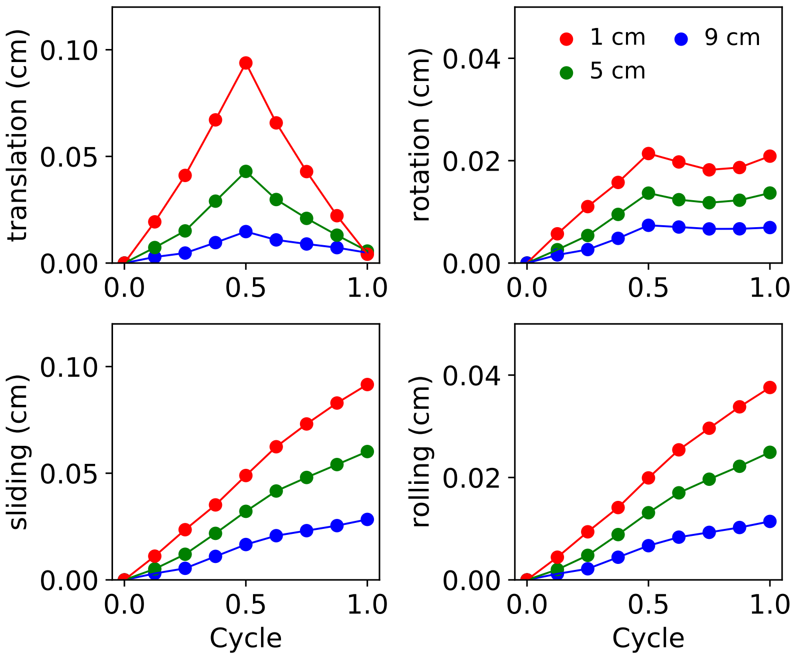


Figure 4. Analogue to Fig. 5 computed in the MD simulations.

## III. CORRECTING TRANSLATIONS ASSUMING LINEAR STRAIN

In Figure 4 of the main text, we observe that the translational motion is heavily biased based on it's distance to the compression wall. This is expected as the beads close to the compression wall feel more force than beads that are at the other end of the container. If we assume a linear relationship between this displacement, we can subtract that bias out of the translations. Figure 5 shows this correction to Figure 4 for the translational displacements along with the rotations. Here, we see translations in the absence of the linear bias follow closely to the rotational displacements. However, we notice a deviation at the extreme ends of the plot, in which there are more rotations than translations. This could be due to the excess amount of sliding displacements we observe deep in the bulk of the material.

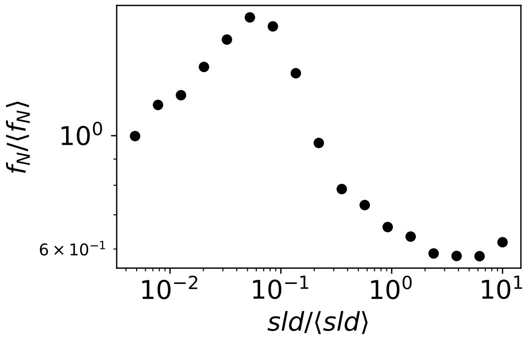


Figure 5. Correlation between sliding displacements and contact forces. Here, the larger amount of sliding displacement corresponds on average to a lower contact force.

## IV. MOLECULAR DYNAMICS SIMULATIONS

We performed the simulations using in-house software called pkdgrav [7]. We integrated the equations of motion in leap-frog fashion to compute changes in particle displacements, velocities, and orientations. Normal forces were calculated with a linear spring constant. Tangential forces were calculated using a spring dashpot model with frictional forces. The time step and spring constant were determined to allow for a $\ll 1\%$ overlap between spheres. The coefficients of static, rolling, and twisting friction were 0.2, 0.01, and 0.001. We use a shape parameter $\beta$ of 0.5.

The simulation's setup is identical to the experimental design: A square container is filled with spheres, each with a diameter of 5 mm and a mass of 0.0618 g. We initialize the material by dropping the spheres into the square container with a uniform downward gravitational force. The container is then shaken twice to help settle the configuration. A top weight of 1 kg is placed on top of the spheres to provide a constant pressure. Compression occurs as one of the container walls moves incrementally. See Ref. [8] for more information about the simulation's setup.

[1] M. Harrington, M. Lin, K. N. Nordstrom, and W. Losert, Granular Matter **16**, 185 (2014).
[2] D. P. Kingma and M. Welling, arXiv (2013), https://arxiv.org/abs/1312.6114.
[3] C. Doersch, arXiv (2016), https://arxiv.org/abs/1606.05908.
[4] W. Zhong, J. M. Gold, S. Marzen, J. L. England, and N. Yunger Halpern, Scientific Reports **11**, 9333 (2021).
[5] W. Kabsch, Acta Crystallographica Section A **32**, 922 (1976).
[6] M. R. Kuhn and K. Bagi, International Journal of Solids and Structures **41**, 5793 (2004).
[7] S. R. Schwartz, D. C. Richardson, and P. Michel, Granular Matter **14**, 363 (2012).
[8] Z. A. Benson, A. Peshkov, D. C. Richardson, and W. Losert, Physical Review E **103**, 062906 (2021).
